# Supplementary material for: GPS-SSL: Guided Positive Sampling to Inject Prior Into Self-Supervised Learning
Source: arXiv:2401.01990 source file (2024-01-09)
Supplement: Supplementary file 1 [file anti-human-trafficking.tex]

\subsection{Introduction to Anti Human Trafficking}
One real-world application that SSL can have a deep impact on is analyzing online images from online markets to uncover fraudulent activities. Since this type of data has a high volume and labelling this data, even if feasible, is highly noisy and expensive, this creates the perfect setting for SSL methods to shine. More specifically, in this paper we focus on the application of SSL methods for countering human-trafficking, in which images of victims in different locations, e.g., hotels, are uploaded to escort websites and advertised.

Forced labor and human-trafficking (HT) are one of the biggest issues of our current society. The International Labour Organization estimates that this industry has an annual profit of \$99 billion worldwide \citep{international2017global}. With the advance of advertisement technology and easy-to-use and low-risk online platforms, traffickers have been exploiting such platforms for recruiting victims, e.g. by posting fake recruitment ads, or soliciting buyers, e.g. by advertising their victims on online escort websites causing the majority of victims to be advertised online \citep{minor2015report}.

Studies on data-driven HT detection rely on discovering certain information from individual or multiple ads that separate them from genuine ads and makes them suspicious of trafficking. Said information could be extracted from the text \citep{nagpal2015entity,li2018detection}, the images used in ads \citep{stylianou2019hotels}, or both \citep{tong2017combating}. 
Although there has been a growing amount of research on anti-HT, most of these studies focus on analyzing the textual data and overlook the images in their analysis \citep{li2018detection}, or fail to effectively incorporate the information form images, e.g. only looking at exact matches \citep{rabbany2018active} or having no performance gain \citep{tong2017combating}. 
Moreover, images can be considered as a group to draw connections between them. For example, if a set of images from different advertisements share a common background or a certain feature in their pictures, these advertisements can be flagged as ``suspicious and organized'' and could be further analyzed by an investigator.

Many image datasets have been proposed in previous literature; however, most of them are not suitable for the mentioned tasks of countering HT. In more detail, most images encountered in this domain contain masked people in different locations, e.g. hotel rooms, and are mostly similar to each other, whether they are taken in the same hotel or not. Hence, the difference between images usually lie in the subtle details of the objects that are present in most images, e.g. bed sheets, and datasets consisting of classes with evidently different objects, e.g. dogs, chairs, airplanes, do not suit this task. For this reason, Hotels-50K \citep{stylianou2019hotels} and Hotel-ID \citep{kamath20212021} were introduced for hotel classification for anti-HT, which contains images of hotel rooms from numerous hotel branches around the world. The datasets additionally provide the hotel chain, i.e., super-class, information for the hotel branches, i.e., classes.

\subsection{Related work on Anti Human Trafficking}

We categorize studies in computer science that are focused on human trafficking (HT), into three main groups: studies detecting HT by analysing individual ads, studies that link multiple ads for uncovering organized activity, and finally, studies that propose counter HT-specific tools, e.g. datasets. We elaborate on these categories in the following sections.

\paragraph{Methods based on individual ad analysis}
Escort ads often contain text and a set of images. One popular line of anti-HT studies focuses on the information in individual ads and aims to classify whether the ads are suspicious of HT or not. These studies mostly merely focus on the textual data \citep{wang2019sex, alvari2016non, dubrawski2015leveraging} and ignore all visual cues. For instance, in \cite{wang2019sex}, the authors analyze the textual data of ads in the Trafficking-10k \citep{tong2017combating} dataset to predict the likelihood of a an ad relating to HT.
In \cite{tong2017combating}, a multi-modal model is proposed that incorporates both the ad text and images for HT detection. Their language network consists of a long short-term memory (LSTM) network 
% to tackle textual challenges, such as the lack of grammatical structures and containing a large amount of irrelevant text
, followed by a fully connected layer to output a text representation. Their vision network consists of a VGG network followed by fully-connected layers to calculate the image representations. Finally, the two type of representations are combined with a third network to detect if an ad is related to HT or not. Although this study uses the images, they mention the vision module does \textit{not} add much to the performance of the model and that the images could potentially be used more efficiently.  
% Specifically, the VGG network takes in at most 5 images, the median number of images per ad in the dataset, and is fine-tuned by being trained to map each of an ad's images to the ad label. After fine-tuning, three fully connected layers are added to the VGG network to complete the vision network, which finally outputs $h_v \in \mathbb{R}^{5\times200}$, the representation of the 5 input images. Finally, the language and vision representations are merged by an outer product, i.e. $h_m = h_l \otimes h_v \in \mathbb{R}^{5\times200\times300}$, to create a multi-modal representation that contains the information from both modalities. The multi-modal representation is finally given as input to a convolutional network to detect if the ad is related to HT or not. However, they mention that the information gained from the language modality is more impactful than the vision modality on the output, and the performance gap of utilizing the text and images compared to only using the text is minimal.

\paragraph{Methods based on linking ads}
Another line of work regarding anti-HT aims to extract features from each ad and link multiple ads together by finding shared features and detect organized activity in a \textit{group} of ads. Most of these studies only use the textual signals to link ads, such as shared phone numbers or bi-grams. For example, \cite{li2018detection} uses unsupervised learning on the textual data in ads to detect groups of ads with similar templates, and further, connect similar templates to identify the signature pattern of organized activities.

There have also been studies that use the hashcodes of the images in the ads, as well as the text, as indicators for linking ads \citep{rabbany2018active, nagpal2015entity}. Nevertheless, by using image hashcodes, only ads with the \textit{exact} same image will be matched, and minimal changes to the image, e.g. cropping or resizing it, will cause the hashcode to be drastically different from the original image hashcode, and hence, go unnoticed according to these algorithms. 

\paragraph{Dataset analysis}
Most supervised and unsupervised methods in deep metric learningx on images use ubiquitous datasets for evaluating their methods, such as the CUB-200-2011 \citep{wah2011caltech} or the ImageNet \citep{deng2009imagenet} datasets. These datasets may be suitable for general applications, but nevertheless, they may not be suitable in applications such as analyzing escort ad images. This is because escort ads are often taken in hotel rooms, where a) classes are not well-defined; and b) the images tend to have more visual components. Hence, they do not provide the a vision model with sufficient information to make predictions.

Trafficking-10k \citep{tong2017combating} dataset, a benchmark dataset for anti-HT studies, which includes the text and images of more than 10,000 trafficking ads labeled with the likelihoods of them being associated with HT is one of the main datasets used in previous studies. Later, a study \citep{stylianou2017traffickcam} presented a fully realized crowdsourcing platform, TraffickCam, that is a database of hotel images and enabled law enforcement investigators to query hotel images. TraffickCam also allows public users to contribute to the database and submit up to four images of the hotel room at which they stay, along with the hotel's information. Interestingly, \cite{stylianou2019hotels} uses TraffickCam and travel websites to collect over a million images from 50,000 hotels from around the world, presenting the Hotels-50K dataset, in order to improve the task of hotel recognition. They collect their hotel images from 91 major hotel chains along with many smaller hotel chains. A subset of this dataset, Hotel-ID \citep{kamath20212021}, was also released, which only contains images from TraffickCam. This smaller dataset compared to the Hotels-50K, contains 7,769 hotels, and also 87 hotel chains.
However, despite being very rich in information, this dataset was originally created for hotel classification; hence, all classes in the evaluation section of it were previously seen by the model during training. Thus, using the standard training/evaluation splits does not reflect the real application scenario, where we can encounter unseen classes.

% Todo: relate it to image linking
% \input{TAB/hyperparams}
% \input{tabs/hotels50-allmetrics}
